# Supplementary material for: Unconditionally Safe Light Client
Source: arXiv:2405.01459 source file (2024-05-02)
Supplement: Supplementary file 1 [file appendix.tex]

\section{Overflow form other sections}
\label{sec:set-diff-dodis}
Goes here.
